# Supplementary material for: Power of Bonus in Pricing for Crowdsourcing
Source: arXiv:1804.03178 source file (2021-10-27)
Supplement: Supplementary file 1 [file supp.tex]

% !TEX root =  main.tex

%\onecolumn
\appendix
\addcontentsline{toc}{section}{Appendices}
\section*{Supplementary Material}
\section{Taxonomy of Related Work}
We classify the existing related work on pricing and incentivization in crowdsourcing by two criteria: forward/reverse auction and posted/non-posted pricing. Each combination is often adopted, depending on the type of crowdsourcing applications or the way of crowdsourcing system is operated. We start by the mechanisms with reverse auction, because this paper lies in the case of reverse auction with posted pricing, followed by those with forward auction.   

\smallskip
\noindent
{\bf \em Reverse auction with non-posted pricing.}
In the mechanisms with reverse auction, a requester tries to procure a set of efforts from workers to maximize its utility under a fixed budget from multiple workers, has widely been studied with emergence of applications like crowdsensing or crowdsourcing platform, also referred to as {\em budget-feasible mechanism design.} \cite{BudgetFeasible:Singer10} firstly defines a problem of budget-feasible mechanism under a prior-free scenario, and proposes a constant-factor approximation mechanism to the optimal one with exact knowledge of workers' cost.\footnote{The outcome of mechanism which exactly knows all workers' cost is called as {\em first-best outcome}. If the mechanism is only aware of the prior distribution of which each worker's cost is realized, the optimal outcome is called as {\em second-best outcome}.} \cite{BudgetFeasible:Bei10} study a budget-feasible mechanism in the Bayesian setting. They provide a constant-factor approximation mechanism to the second-best outcome under the subadditive utility function by exploiting a prior-free mechanism as a sub-routine. 
There exists a series of work which studies a mechanism with budget constraint to model the crowdsourcing applications using the concept of sequential game \cite{Sealedbid:Zheng17,Sealedbid:Zhang,Sealedbid:Zhang2,Sealedbid:Gan}.
To avoid the computational intractability of an optimal winning bid
allocation for maximizing the utility, they suggest a
greedy-style mechanism, and prove its truthfulness, individual
rationality, and frugality.

% \begin{comment}
% \begin{table}[t!]
% \caption{Related work: CS (CrowdSourcing)}
% %\vspace{-0.3cm}
% \centering
% \begin{tabular}{c c c c}
%   \hline\hline
%   Major CS app.  &Model &Paper\\
%   \hline
  
% Contest  &All-pay auction &\cite{Allpay:Cavallo12, Allpay:Chawla15,Allpay:Dipalantino09,Allpay:Xu17} \\

%   \hline
%   Ecommerce &Sealed-bid auction & \cite{Sealedbid:Gan,PricingisDifficult:Gao,Sealedbid:Zhang2,Sealedbid:Zhang,Sealedbid:Zheng17} \\
  
%   \hline
%   Microtask&Posted price & \cite{BudgetFeasible:Anari13, Posted:Balkanski16, Posted:Sun14, Posted:Hu17, Posted:Han16, OnlinePosted:Singla13, OnlinePosted:Han17} \\
  
%   \hline
% Microtask&Misc. &  \cite{Eliciting:Liu16,Eliciting:Radanovic16,Axiomatic:Shahnips,Axiomatic:Shahicml} \\

%   \hline
 
% \end{tabular}
% \label{tab:Rel}
% \vspace{-0.3cm}
% \end{table}
% \end{comment}

\smallskip
\noindent
%{\bf \em Budget-feasible Posted Pricing.}
{\bf \em Reverse auction with posted pricing.}
With semantics of {\em first-come-first-served} and {\em while-supplies-last}, posted pricing has largely been explored due to its simplicity and practicality on real-world applications. 
\cite{Posted:Bad12} propose a budget-feasible posted pricing with constant-factor approximation, assuming online worker arrivals.
\cite{BudgetFeasible:Anari13} also study the same problem with an improved approximation ratio under a large-market assumption. Note that the both papers are based on competitive performance to first-best outcome under prior-free online scenario.
\cite{Posted:Balkanski16} studies a budget-feasible posted pricing problem in Bayesian offline setting, and prove that such pricing is able to closely approximate the Bayesian optimal mechanism, i.e. the second-best outcome, for large markets assuming submodular objective. \cite{Posted:Han16} consider a problem which is dual to the Bayesian budget-feasible posted pricing problem in offline setting, wherein, given utility constraint, the goal is to minimize cost. \cite{OnlinePosted:Han17} study a similar problem, but for homogeneous workers and heterogeneous tasks setting. Our work derives from the branch of Bayesian budget-feasible posted pricing problem in offline setting, as a variant of the original model with a concept of bonus function.

%\note{forward/posted pricing}
\smallskip
\noindent
%\note{forward/non-posted pricing}
%{\bf \em Crowdsourcing as Forward Auction. }
\noindent {\bf \em Forward auction with non-posted pricing.}
Crowdsourcing has also been studied under the setting of forward auction \cite{OptimalAuction:Myerson}. 
All-pay auction has been studied as a proper model
for crowdsourcing contest like Kaggle (different from Microtask as in this paper), where all workers obligatorily pay their bids (i.e.,
efforts) regardless of the allocated items, and then get paid from the
task requester based on their bids \cite{Allpay:Dipalantino09,Allpay:Chawla15,Allpay:Cavallo12}. They propose the algorithms with
a certain approximation ratio of various bidding strategies, for
different forms of revenue functions, targeting a various application of crowdsourcing contests. 
\cite{PricingisDifficult:Gao} consider the hardness in the verification
of submitted quality and propose a cost-effective mechanism with
guaranteed symmetric Nash Equilibrium. Large branches of work in combinatorial auction can also be applied to crowdsourcing platform by grouping the tasks and allocating the subset of tasks to proper workers \cite{Combi:Xu17,Combi:Guru05}.

\smallskip
\noindent{\bf \em Forward auction with posted pricing.}
\cite{Posted:Chawla09} and \cite{Posted:Yan11} prove that posted pricing can at least half as good as optimal auction for a single-item environment.
\cite{Posted:Zhang17} reveal that the online cloud resource problem can be expressed nicely by a posted pricing mechanism in online setting, showing its equivalence to a variant of an online knapsack problem and proposing an optimal posted pricing mechanism in terms of the competitive ratio.
Other types of on-line setting for posted pricing have also been studied,
where the requester gradually adapts to heterogeneous worker qualities or task difficulties. \cite{VariantPosted:Singer13} consider online worker arrivals with the objective of maximizing the number of solved tasks. \cite{Posted:Hu17} and \cite{OnlinePosted:Singla13} study this problem in the context of posted pricing for crowdsensing platforms. They again assume online arrivals of heterogeneous workers and  formulate a problem in the multi-armed bandit framework, providing analysis of the UCB (Upper Confidence Bound) algorithm.

\smallskip
\noindent
{\bf \em Position of this paper.} This paper lies in the case of reverse auction with posted pricing, where our main applications include microtasks in the crowdsourcing platform, e.g., a spell correction task of a document. 
Different from the prior work in this setup, whose main interest lies in finding a constant-factor approximation mechanism, our focus is more on quantifying the utility gap between personalized and common pricing and analyzing the gain coming from bonus payments. We prove that a simple bonus plays a key role of significantly reducing the gap between those two, implying that a simple pricing is also efficient. We conclude this section by presenting a list of related work on bonus payment.  

\smallskip
\noindent
{\bf \em Bonus payment for workers.}
There exists an array of prior work studying the concept of bonus from various angles. 
The problem of designing a bonus to a worker based on her work quality has massively been studied in economic literature as a name of contract theory. The contract theory, whose basic form is formulated by a game between a single worker and a single company, studies how to write a contract to the worker to achieve a maximum revenue. 
In a complete information scenario, it is known that a convex programming optimally solves the problem \cite{Contract:Grossman83}. \cite{Contract:Carroll15} proves that a linear contract is optimal under some assumption in moral hazard scenario. In this context, designing an efficient bonus payment in crowdsourcing applications can also be regarded as a variant of contract theory. However, the problem naturally differs from our work, since the requester needs to allocate the resource not only within a worker, but also among the workers.
Regarding a performance-based bonus mechanism to the sequence of workers,
\cite{Bonus:Yin15,Bonus:Ho15} conduct a massive real-world experiment to measure the performance of various pricing mechanisms with bonus. \cite{Eliciting:Liu16} and \cite{Eliciting:Radanovic16} design a truthful incentive mechanism assuming that workers try to align their output together, and analyze an equilibrium of the system. \cite{Axiomatic:Shahnips} and \cite{Axiomatic:Shahicml} redefine the concept of
truthfulness, and propose an axiomatic approach to find a truthful mechanism by consecutively offering a contract to a single worker.

\section{Evaluation}

\subsection{Simulation}
In order for verifying the analytical result and giving insights on designing pricing policy, we provide numerical evaluation of different pricing policies with heterogeneous bonus structure.
% numerically investigate expected utility in different pricing policies with heterogeneous bonus structure,
%
%\smallskip
%\noindent
%{\bf \em Setup.} 

\smallskip
\noindent
{\bf \em  Efficiency of common pricing with bonus.} 
We consider the utility function $u(  \vec{s} \circ \vec{x}) = \sum_{i \in \set{N}} s_i x_i $,
budget $B = 3$, and $n = 16$ workers partitioned into two disjoint groups. 
Each worker's profile is independently drawn from 
type~1 distribution: $(s,c) = (0.1, 0.5)$ and $(s,c) = (0.66, 0.6)$ with equal probabilities if included in the first group;
or type~2 distribution: $(s,c) = (0.1, 0.5)$  and $(s,c) = (1, 0.8)$ with equal probabilities otherwise.
Note that type~2 is more efficient than type~1 on average.
In Figure~\ref{fig:util}, 
we compare utilities under the following five pairs of pricing and budget: 
%\begin{enumerate}[(C1)]
(C1) common pricing $\linear(\alpha_B) = (0,\alpha_Bu_0(s_i))$ with budget $B$; 
(C2) the same policy of (C1) with budget increased to $1.4B$; 
(C3) the optimal common pricing without bonus for budget $B$, i.e., any common pricing without bonus cannot have utility larger than this;
(C4) the personalized pricing $\vec{\pi}_p(\vec{\beta}_B) = [(\beta_{B,i}, 0)]$ with budget $B$; and 
(C5) the oracle pricing policy, which knows the worker profiles and arrival order in advance, and maximizes utility as \textbf{Oracle} does, with budget $B$.
%\end{enumerate}[C1]
%(C1) , (C2) the same as (C1) but budget increased to $1.4B,$ 
%(C3) the optimal common pricing without bonus for budget $B$, 
%(C4) personalized pricing $\vec{\pi}_p(\vec{\beta}_B) = [(\beta_{B,i}, 0)]$ under budget $B$, and 
%(C5) the oracle pricing policy, i.e., the worker profiles are public and the requester posts the price 
%in per-incidence manner as in \textbf{Oracle}, under budget $B$.
%We also consider two different worker arrival orders: (i) type~1 workers first and then type~2 ones, and (ii) the other way around.  

In Figure~\ref{fig:util}, comparing (C1) to (C3) and (C4), the simple choice of common pricing with bonus in (C1)
drastically outperforms (C3) and (C4), which use optimal common pricing or personalized pricing but no bonus. This shows the importance of employing bonus and coincides with Theorem~\ref{thm:pad_bonus}. In addition, the utility of (C1) is comparable to the oracle one of (C5), while in order to achieve the oracle utility of (C5), additional budget is required but not much as $40\%$ since the common policy of (C2) with budget $1.4B$ outperforms the oracle of (C5) with budget $B$. This hence suggest that using common pricing with bonus can be sufficient.

%the oracle pricing policy of (C5) outperforms the others except (C2) with extra budget. 
%Comparing (C1) and (C5), we observe that the impact of bonus is much more significant than that of personalization. 
%The expected utility of (C2) exceeds that of (C3), implying that it would be more helpful to augment the budget slightly under a simple pricing than to spend the budget on collecting individual profile distributions and then apply a complex pricing. 
%As stated in Theorem~\ref{thm:pad_bonus}, the utility of (C4) is extremely low, since there exists no device to filter out poor workers, i.e. worker with $(s,c) = (0.1,0.5)$.
%Note that, in case of arrival orders of Type 1 first and Type 2 next, 
%where inefficient workers come ahead of efficient ones, the utility of (C4) becomes smaller
%due to the lack of power of discriminating workers based on their qualities. 

\begin{figure*}[!t]
    \centering
    % 	\hspace{0.1em}
        \subfloat[PoA and PoB]{\includegraphics[width=0.25\columnwidth]{fig/bar_graph.eps}\label{fig:util}}
        \hspace{0.1em}
        \subfloat[Expected utility under different bonus structure]{\includegraphics[width=0.27\columnwidth]{newfig/typeutility}\label{fig:typeutility}}
        \hspace{-0.7em}
        % \vspace{-1em}
        \subfloat[Type $1'$ distribution]{\includegraphics[width=0.24\columnwidth]{newfig/type1}\label{fig:type1}}
        \hspace{-0.7em}
        \subfloat[Type $2'$ distribution]{\includegraphics[width=0.24\columnwidth]{newfig/type2}\label{fig:type2}}
    \caption{(a) Utilities of five choices of pricing and bonus (C1-C5); (b) Utility vs. common pricing with varying bias and bonus; (c) and (d) worker profile distributions used for (b) where darker red indicates higher density of distribution.}
\end{figure*}

\smallskip
\noindent
{\bf \em A guide to design good pricing policy.} 
%In the conjunction with the analytical results in Section~3, 
We further provide a numerical study on the impact of the design choice in common pricing. 
% the structure of efficient pricing to obtain practical insights and guidelines on the design of pricing policy. 
To this end, we use the same setup for Figure~\ref{fig:util} but 
use different profile distributions
type~$1'$ and type~$2'$ shown in Figures~\ref{fig:type1}~and~\ref{fig:type2}, , respectively,
instead of type~$1$ and type~$2$. 
% only difference of worker profile distributions. Here, each worker $i$'s private values $c_i$ and $s_i$ are correlated as in Figures~\ref{fig:type1} or \ref{fig:type2} with the same proportion, 
We consider a form of common pricing with base $nP/B$ for $P = 0,0.075, \ldots 0.75$ and bonus $q(s_i) = k \cdot s_i^\rho$, where $k$ is constant and $\rho \in \{0.3,0.6,\ldots, 3\}$ is bonus-parameter. 
We adopt a quadratic utility $u(s_1,s_2,\ldots,s_n) = \sum_i s_i^2$.
Figure~\ref{fig:typeutility} shows the expected utility of pricing $(p,q(s_i)) = (p, k_{p}^\star s_i ^{\rho})$, where for each value of base payment $p$ and $\rho$, the optimal parameter $k_p^\star$ is searched exhaustively, whose interpretations are as follows: 

\smallskip
\begin{compactitem}[$\circ$]
\item {\em Ratio of base to bonus:}
If $\rho \leq 1.8$, as the base payment increases, the expected utility decreases, so that there exists no benefit of exploiting base payment. In otherwise, imposing a certain amount of base payment plays a role if $\rho$ becomes higher. It can be interpreted as, given a proper structure of bonus function, applying only the bonus payment with proper constant would be sufficient to optimize utility. However, if the bonus structure is badly designed, e.g. $\rho = 2.7, 3.0$, the base payment plays rather a critical role. In finding optimal pricing, we expect that paying a certain amount of base payment would help regardless of bonus structure in many cases, since it makes possible to recruit a large number of low-quality workers in low-cost, where the requester becomes possible to exhaust given budget entirely.
\vspace{0.1cm}
\item {\em Structure of bonus:}
The requester utility is optimized near the region $\rho = 2$ where we remind that the utility is quadratic function.
To achieve higher utility, the requester needs to recruit the workers who possess larger amount of utility-to-cost ratio, i.e. $\frac{u_0(s_i)}{c_i}$. Hence in quadratic utility case, the requester utility would be optimized if it tries to recruit more workers with larger $\frac{s_i^2}{c_i}$, which leads to highest utility near in $\rho = 2$. We expect that given a separable utility function, one can nearly optimize requester utility by imposing bonus payment with structure $k \cdot u_0(s_i)$.
\end{compactitem}

\subsection{Experiment details}
\begin{figure*}[!t]
    \centering
        \subfloat[The typo correction task used in the experiment]{\includegraphics[width=0.45\columnwidth]{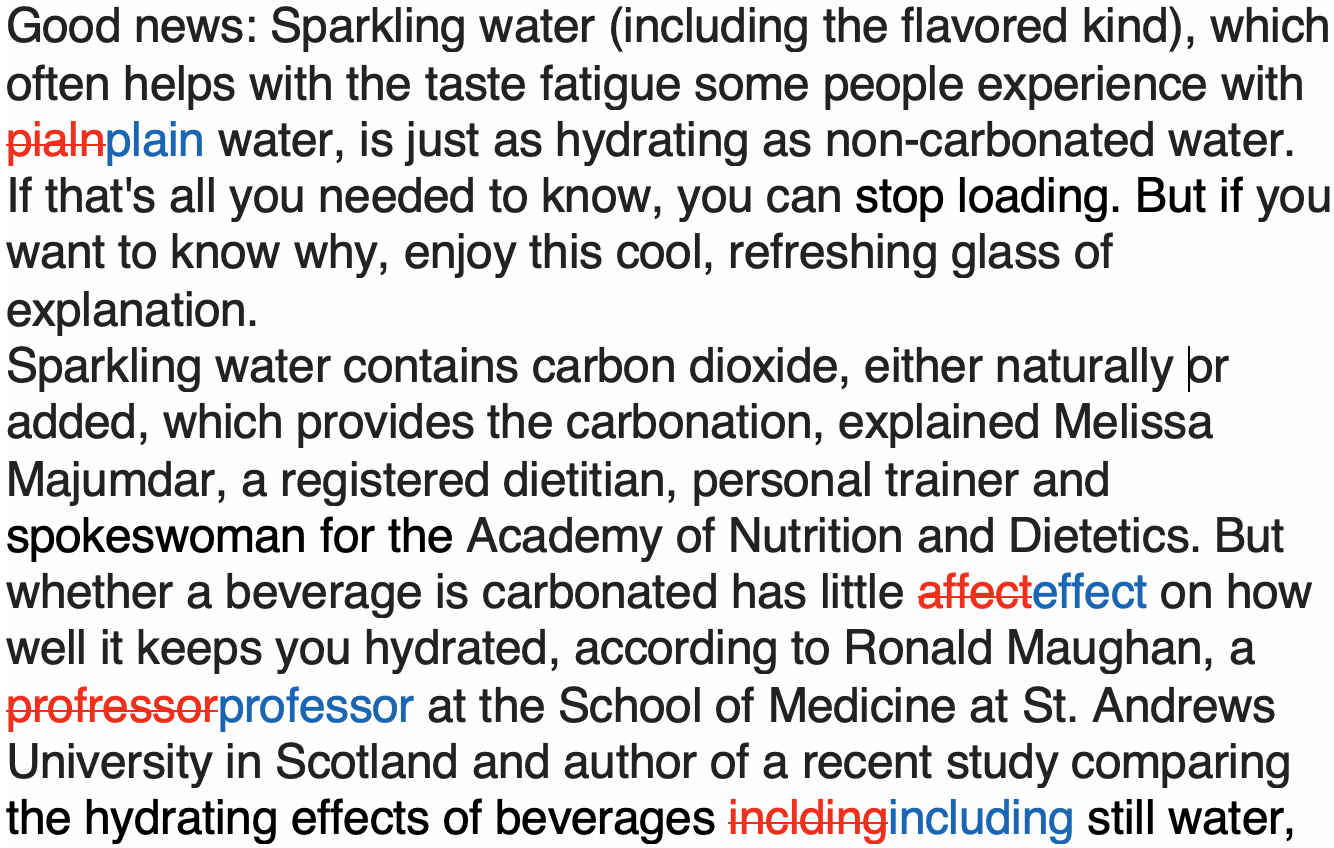}\label{fig:corrected}}
        \hspace{0.1em}
        \subfloat[The actual display of task to workers ]{\includegraphics[width=0.53\columnwidth]{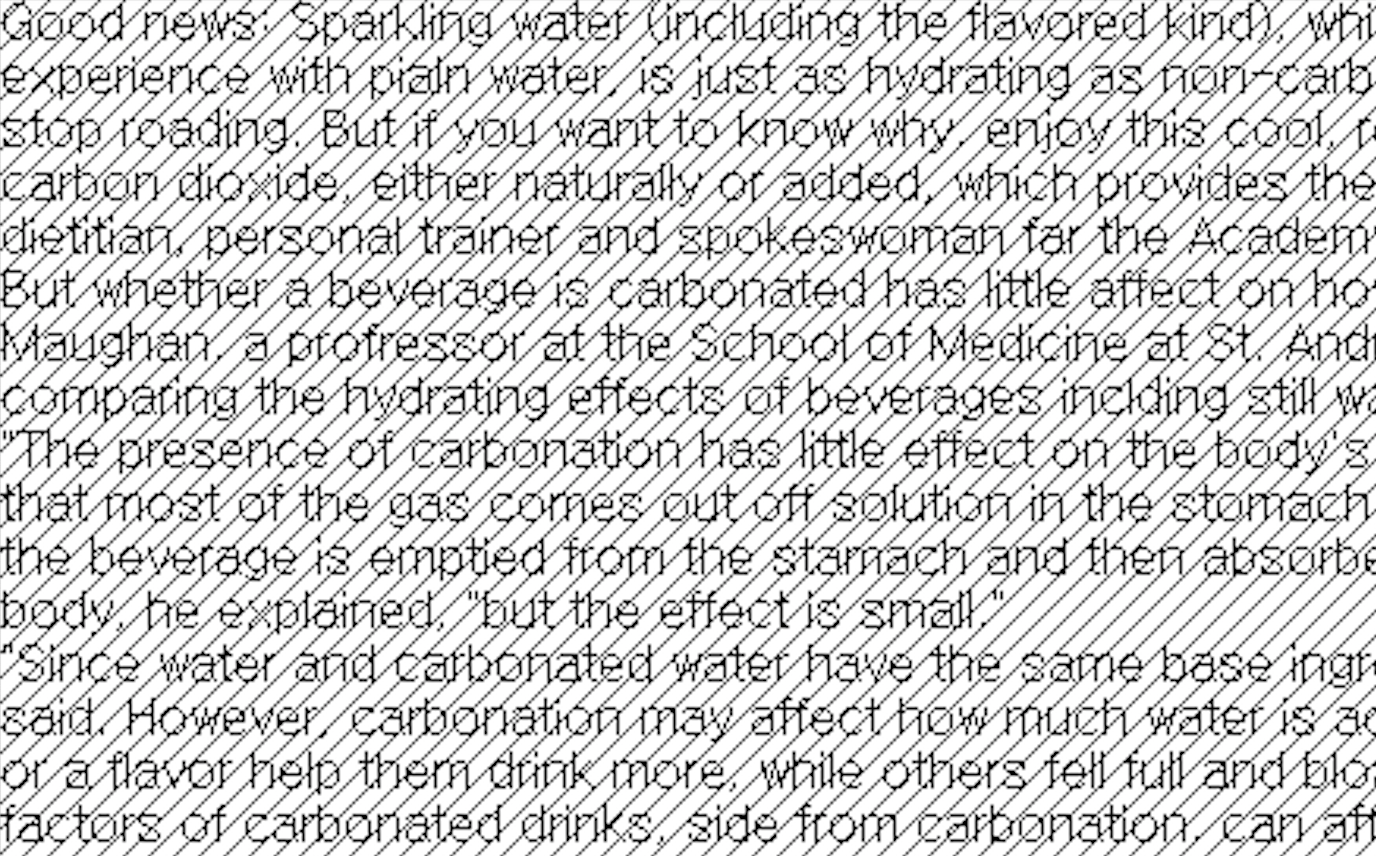}\label{fig:task}}
    \caption{(a) The typo correction task used in the experiment, which we
    generated based on an article in \protect\cite{CNNarticle} by inserting typos highlighted in red
    instead of original words shown in blue; and
    (b) display shown to workers with dashed lines to prevent to use of automated tools.}
    \label{fig:task_detail}
\end{figure*}

In what follows, we provide a detailed explanation on real-world experiment. In Figure~\ref{fig:task_detail}, we present the task we posted in Mturk for workers to solve. In Figure~\ref{fig:corrected}, we borrow an article from CNN~\cite{CNNarticle}, and alter some words in the articles into hand-made typos, i.e. we change the blue-colored words into red-colored words.
The typos are almost evenly distributed over the article, and for each target word, we alter it into an elementary level of typo so that there exists no fundamental difficulty in correcting the typos whenever the worker discovers it. 
When posting the task in Mturk platform, we intentionally put dashed lines in the display of the article in order to prevent the workers to exploit some automated tools, like OCR, and to provide the answers without exerting their own effort. To choose a proper price for our task, we presume that normal workers would spend about $5$ to $10$ minutes in working on task, and decide the base and bonus payment so that the expected payment divided by spent time stays near in minimum wages.

We now provide the details of how we model and compute {\em simulated OPP}.
We first assume that the workers are sampled from i.i.d. joint distribution where $c_i \sim \text{Uniform}(\{0.1, 0.2, \ldots, 2.0\})$, and $s_i \sim \set{N}(xc_i+y, z^2)$, and they arrive with geometric distribution $G(\lambda)$ for some hidden parameters $x,y,z,\lambda>0$.
To infer $x$ and $y$, we compute expected quality for every {\bf $b$-base} policy where $b\in \{0.1,0.3,0.5,0.7\}$, and then use linear regression over $b$ and expected quality, which leads us to obtain $x=2,y=7,$ by assuming $b=c_i$\footnote{In this way, the quality distribution will be overestimated since the workers accepting {\bf $b$-base} policy will actually possess cost higher than $b$. Eventually, this leads to an overestimation of utility, and finally will result a conservative comparison between utility of OPP and common pricing policies, i.e. the actual utility gap might be much lower }. We obtain $z=4$ by computing the expectation of standard deviation for every {\bf $b$-base} policy. Finally, we get $\lambda=0.13$ by computing expected arrival interval between any two consecutive workers for every {\bf $b$-base} policy.
Given this model, we first assume that the total budget $B$ is $14$ as in the total consumed budget in $0.7$-base policy. Then, we sample $65$ data from the profile distribution and their arrival time from arrival model, and compute utility at each time of OPP($14$) computed from this sample. Finally, we repeat this process 100 times to estimate an expected performance over worker profile and arrival samples.
